# Supplementary material for: About some works of Boris Polyak on convergence of gradient methods and their development
Source: arXiv:2311.16743 source file (2024-12-24)
Supplement: Supplementary file 1 [file 4_appendix.tex]

\renewcommand{\theequation}
% {П.\arabic{equation}}
% \section*{{$\qquad \qquad \qquad \qquad \qquad \qquad \qquad \qquad \qquad$\itПРИЛОЖЕНИЕ} } \label{sec:apCATD}

% \section{Раздел приложения 1}
    % Текст приложения...
%=========== the end of Appendix A: Раздел приложения 1 ==========
